# Supplementary material for: Testing strong exogeneity in proxy SVARs with internal synthetic proxies
Source: arXiv:2610.36093 source file (2026-12-01)
Supplement: Supplementary file 1 [file Appendix.tex]

\PassOptionsToPackage{dvipsnames}{xcolor}
\documentclass[12pt]{article}
\usepackage[pass]{geometry}

%\usepackage{natbib} %Literatur
%\usepackage{chicago} %Literatur
\usepackage{graphicx} %Graphen
\usepackage{subfigure} %Abbildungen
\usepackage{lscape}	%Gedrehte Darstellungen
%\usepackage[latin1]{inputenc} %Umlaute
\usepackage{pst-plot, pstricks} %Graphen
\usepackage{fancybox,amssymb,color} %Fancy stuff (z.B. Umrahmungen), Formeln, Farben
%\usepackage[british,UKenglish,ngerman]{babel} %Sprache
\usepackage[english]{babel}
%\usepackage{bibgerm} %Deutsche Abkürzungen
\usepackage{setspace} %Zeilenabstand
\usepackage{epstopdf}
\usepackage[capposition=top]{floatrow} 
\usepackage{float}
%\usepackage{hyperref} 
\usepackage{enumitem}
\usepackage{longtable}
\usepackage{tabularx,calc}
\usepackage{multirow}
\usepackage{booktabs}
%\usepackage{acro}
\usepackage{setspace}
\usepackage{lscape}
\usepackage{mathtools}
\usepackage{rotating} 
% PSTricks and adjustbox both define \clipbox; use the adjustbox implementation.
\let\clipbox\relax
\usepackage{adjustbox}
\usepackage{blkarray}
	
\usepackage[authoryear]{natbib}
\bibliographystyle{chicago} % Shared bibliography style.

%\usepackage[demo]{graphicx}
\usepackage{caption} 
%\usepackage{subcaption}

%\usepackage{amsmath} %Formeln
%\usepackage{wasysym}
%\usepackage{amssymb}

\usepackage{amsmath}
%\usepackage{wasysym}
\usepackage{amsthm} 
\usepackage{amssymb}
\usepackage{amsbsy}
\usepackage{bm}

% Einstellung zum Seitenlayout: 
\pagestyle{plain} %Seitenkopf leer, Fußzeile mit zentrierter Seitennummer 
%\setlength{\parskip}{1ex} %Abstand zwischen Absätzen
%\topmargin-20pt \oddsidemargin0pt \evensidemargin0pt %\textheight665pt
%\textwidth420pt \marginparwidth0pt %Seitenabstände
% \linespread {1.5}

\addtolength{\oddsidemargin}{-.5in}%
\addtolength{\evensidemargin}{-1in}%
\addtolength{\textwidth}{1in}%
\addtolength{\textheight}{1.7in}%
\addtolength{\topmargin}{-1in}%

\doublespacing



\newenvironment{mybsmallmatrix}
{\hbox\bgroup
	\delimiterfactor=1000
	\delimitershortfall=0pt
	$\left[\smallmatrix}
{\endsmallmatrix\right]$\egroup}

\DeclareMathOperator*{\argmin}{arg\,min}


\usepackage{changes}%added
\definechangesauthor[name={Sascha}, color=green]{Sascha}

\newtheorem{proposition}{Proposition} 
\newtheorem{lemma}{Lemma} 
\newtheorem{corollary}{Corollary} 
\newtheorem{assumption}{Assumption} 
\newtheorem{definition}{Definition} 
\setlength{\parindent}{0em} 
 
% --- BEGIN (shu's addition)-- & 
\usepackage[dvipsnames]{xcolor}

\newcommand{\one}{\mathbb{I}}
%% --- comment
\newcommand{\sw}[1]{\textit{\textcolor{cyan}{#1}}}
\renewcommand{\blue}[1]{\textcolor{blue}{#1}}
\renewcommand{\red}[1]{\textcolor{red}{#1}}
%% --- edit 
%\newcommand{\rev}[1]{\textcolor{orange}{#1}} % change the col before submission (!)
%\newcommand{\rev}[1]{\textcolor{black}{#1}} % uncomment this before submission (!)

% Shortcut for bold text in math mode, e.g. $\b{X}$
\let\b\mathbf

% Shortcut for bold Greek letters, e.g. $\bg{\beta}$
\let\bg\boldsymbol

% Shortcut for calligraphic script, e.g. %\mc{M}$
\let\mc\mathcal
\let\bs\boldsymbol

% Convergence: right arrow with optional text on top
% E.g. $\converge[p]$ for converges in probability
\newcommand{\converge}[1][]{\xrightarrow{#1}}

% Weak convergence: harpoon symbol with optional text on top
% E.g. $\wconverge[n\to\infty]$
\newcommand{\wconverge}[1][]{\stackrel{#1}{\rightharpoonup}}

% Independent and identically distributed random variables
% E.g. $ X_1,...,X_n \iid \normal{0}{1}$
\newcommand{\iid}{\stackrel{\smash{\text{iid}}}{\sim}}

% Math. SymbolabkÃ¼rzungen
\newcommand{\betab}{\boldsymbol{\beta}}
\newcommand{\etab}{\boldsymbol{\eta}}
\newcommand{\mub}{\boldsymbol{\mu}}
\newcommand{\thetab}{\boldsymbol{\theta}}
\newcommand{\varepsilonb}{\boldsymbol{\varepsilon}}
\newcommand{\omegab}{\boldsymbol{\omega}}

%\newcommand{\iiddist}{\stackrel{iid}{\sim}}
\newcommand{\vect}[1]{\mathrm{vec}\left( {#1} \right)}
\newcommand{\vech}[1]{\mathrm{vech}\left( {#1} \right)}
%\newcommand{\diag}[1]{\text{diag}\left( #1\right)}
\newcommand{\upb}[1]{\overline {#1} }
\newcommand{\lowb}[1]{\underline {#1} }

% Math mode symbols for common sets and spaces. Example usage: $\R$
\newcommand{\R}{\mathbb{R}}	% Real numbers
\newcommand{\C}{\mathbb{C}}	% Complex numbers
\newcommand{\Q}{\mathbb{Q}}	% Rational numbers
\newcommand{\Z}{\mathbb{Z}}	% Integers
\newcommand{\N}{\mathbb{N}}	% Natural numbers
\newcommand{\F}{\mathcal{F}}	% Calligraphic F for a sigma algebra
\newcommand{\El}{\mathcal{L}}	% Calligraphic L, e.g. for L^p spaces
\newcommand{\D}{\mathcal{D}}

% Math mode symbols for probability
\newcommand{\pr}{\mathbb{P}}	% Probability measure
\newcommand{\E}{\mathbb{E}}	% Expectation, e.g. $\E(X)$
\newcommand{\var}{\text{Var}}	% Variance, e.g. $\var(X)$
\newcommand{\cov}{\text{Cov}}	% Covariance, e.g. $\cov(X,Y)$
\newcommand{\corr}{\text{Corr}}	% Correlation, e.g. $\corr(X,Y)$
\newcommand{\B}{\mathcal{B}}	% Borel sigma-algebra

% Other miscellaneous symbols
\newcommand{\tth}{\text{th}}	% Non-italicized 'th', e.g. $n^\tth$
\newcommand{\Oh}{\mathcal{O}}	% Big-O notation, e.g. $\O(n)$
\newcommand{\1}{\mathds{1}}	% Indicator function, e.g. $\1_A$

% Additional commands for math mode
\DeclareMathOperator*{\dv}{d\!}			% Non-italicized 'with respect to', e.g. $\int f(x) \dv x$
\DeclareMathOperator*{\diag}{diag}		% Diagonal of a matrix, e.g. $\diag(M)$
\DeclareMathOperator*{\trace}{tr}		% Trace of a matrix, e.g. $\trace(M)$
\DeclareMathOperator*{\supp}{supp}		% Support of a function, e.g., $\supp(f)$
\DeclareMathOperator*{\rank}{rank}


% New Assumption with custom numbering of assumptions
\newtheorem{assumptionalt}{Assumption}[assumption]
\newenvironment{assumptionp}[1]{
  \renewcommand\theassumptionalt{(#1)}
  \assumptionalt
}{\endassumptionalt}
\newtheorem{remark}{Remark}
% box for notes
\usepackage[most]{tcolorbox}
\newtcbtheorem{Notes}{\bfseries Notes}{enhanced,drop shadow={black!50!white},
  coltitle=black,
  top=0.3in,
  attach boxed title to top left=
  {xshift=1.5em,yshift=-\tcboxedtitleheight/2},
  boxed title style={size=small,colback=Apricot}
}{notes}
\newtcolorbox[auto counter]{notes}[1][]{title={\bfseries Notes~\thetcbcounter},enhanced,drop shadow={black!50!white},
  coltitle=black,
  top=0.3in,
  attach boxed title to top left=
  {xshift=1.5em,yshift=-\tcboxedtitleheight/2},
  boxed title style={size=small,colback=Apricot},#1}

\newcommand*\dd{\mathop{}\!\mathrm{d}} % d for integrals
% --- END (shu's addition)-- & 
 




% Both document drivers use these identical packages, macros, layout, and spacing.
\usepackage{xr}




\title{Online Appendix for ``Testing strong exogeneity in proxy SVAR with internal synthetic proxies''}
\author{Sascha A. Keweloh \and Shu Wang}
\date{\footnotesize{October 14, 2026}}
\begin{document}
\maketitle
\thispagestyle{empty}






\clearpage
\bibliography{literatur}
\end{document}
